# Supplementary material for: Human Evaluation of Procedural Knowledge Graph Extraction from Text with Large Language Models
Source: arXiv:2412.03589 source file (2024-11-27)
Supplement: Supplementary file 1 [file old-appendix.tex]

\section{Prompts}
\label{sec:app-prompts}

In this section we list all the 7 prompts that build our pipeline for procedural knowledge graph extraction from text (Listings \labelcref{listing:P1,listing:P2,listing:P3,listing:P4,listing:P5,listing:P6,listing:P7}).
The text of the example procedure (\emph{Clean a Computer Keyboard}), and the intermediate examples, can be found on the GitHub repository.

\begin{lstlisting}[
    basicstyle=\ttfamily\scriptsize, frame=single, caption={Prompt 1.}, label={listing:P1},  basicstyle=\scriptsize\ttfamily,frame=single, escapeinside={+}{+}, firstnumber=auto, showstringspaces=false, belowcaptionskip=0em] 
As an expert in information extraction, please, find all relevant steps of a 
procedure. A procedure consists of some steps that, if executed, contribute to 
achieve a goal. A step of a procedure is an instruction that describes an 
action that someone needs to perform. 

Let's use an example: 

{keyboard_example}
We think about which are all the steps of the procedure. 
Let's make a first draft of the steps, in json format:
{keyboard_initial_steps}

The example ends here. 

Extract steps from the following text, using the same json structure as 
in the example. 
{procedure_for_llm}
\end{lstlisting}

\begin{lstlisting}[
    basicstyle=\ttfamily\scriptsize, frame=single, caption={Prompt 2.}, label={listing:P2},  basicstyle=\scriptsize\ttfamily,frame=single, escapeinside={+}{+}, firstnumber=auto, showstringspaces=false, belowcaptionskip=0em] 
You are an expert in procedures and steps, and understanding what is a step 
and what is not. Please, think step by step and check if the steps you 
previously identified are actual steps, or not.   

A procedure may contain, together with a list of steps, additional 
sentences that provide some tips, warnings, comments, tools to be 
used during the step, and that do not describe an action to be performed, 
thus they are not steps.  

A step should contain an action to perform, however, in some cases, even if 
including an action, some sentences are not steps, for example: 

"do not do this" is not an actual step
"be careful not to do this" is not an actual step
"pay attention not to do this" is not an actual step
"you may want to do this" is not an actual step
"you may do this" is not an actual step

Let's use an example. 

From the steps I previously extracted 
{keyboard_initial_steps} 
I check if they are correct, or not, and add the validation and reason 
in the json: 
{keyboard_correct_incorrect} 

The example ends here.  

Think step by step.  
Check if the steps you previously identified are actual steps, or not, 
and provide a reason for your choice. 
Add the validation and reason in the json.
{initial-steps}
\end{lstlisting}

\begin{lstlisting}[
    basicstyle=\ttfamily\scriptsize, frame=single, caption={Prompt 3.}, label={listing:P3},  basicstyle=\scriptsize\ttfamily,frame=single, escapeinside={+}{+}, firstnumber=auto, showstringspaces=false, belowcaptionskip=0em] 
Now it is time to remove from the json all the dictionaries including steps 
that have been annotated as incorrect.  

Let's use an example. 

From the steps I previously extracted
{keyboard_correct_incorrect}
I remove all incorrect steps from the json: 
{keyboard_remove_incorrect} 

The example ends here.  

Remove the incorrect steps from your json output, and remove the validation 
and reason keys from the other steps.  
{correct-incorrect-steps} 
\end{lstlisting}

\begin{lstlisting}[
    basicstyle=\ttfamily\scriptsize, frame=single, caption={Prompt 4.}, label={listing:P4},  basicstyle=\scriptsize\ttfamily,frame=single, escapeinside={+}{+}, firstnumber=auto, showstringspaces=false, belowcaptionskip=0em] 
Now, you have to number the steps, based on their order, and add the 
order number of each step in the output. 

Let's use an example. 

To the steps I previously extracted 
{keyboard_remove_incorrect} 
I add the order number to the json: 
{keyboard_order} 

The example ends here.  

Number the steps of your json output.  
{only-correct-steps} 
\end{lstlisting}

\begin{lstlisting}[
    basicstyle=\ttfamily\scriptsize, frame=single, caption={Prompt 5.}, label={listing:P5},  basicstyle=\scriptsize\ttfamily,frame=single, escapeinside={+}{+}, firstnumber=auto, showstringspaces=false, belowcaptionskip=0em] 
Now, we want to find the tools explicitly mentioned in all the steps we 
identified. By tool I mean any kind of object needed to perform the action 
described in the sentence of the step. Include the name of the tool or tools, 
separated by a semicolon if they are more than one. 
Do not include any entry if no tool is explicitly mentioned.   

Let's use an example.  

In the steps I previously extracted  
{keyboard_order}
I check if any tool is mentioned, and add it to the json  
{keyboard_tools}  

The example ends here.   

Find the tools explicitly mentioned in the steps of your output, and add 
them to the json, if any.
{ordered-steps}  
\end{lstlisting}

\begin{lstlisting}[
    basicstyle=\ttfamily\scriptsize, frame=single, caption={Prompt 6.}, label={listing:P6},  basicstyle=\scriptsize\ttfamily,frame=single, escapeinside={+}{+}, firstnumber=auto, showstringspaces=false, belowcaptionskip=0em] 
Now, we want to find the actions explicitly mentioned in all the steps 
we identified. The action should be expressed as a verb, and it is the action 
that the sentence of the step says to perform. 
A step should have at least one action. If a step includes more than one 
action, include them separated by a semicolon. 

Let's use an example.  

In the steps I previously extracted  
{keyboard_tools}
I check the actions that are mentioned, and add them to the json
{keyboard_actions}  

The example ends here.   

Find the actions in the steps of your output, and add them to the json.   
{tools-steps}  
\end{lstlisting}

\begin{lstlisting}[
    basicstyle=\ttfamily\scriptsize, frame=single, caption={Prompt 7.}, label={listing:P7},  basicstyle=\scriptsize\ttfamily,frame=single, escapeinside={+}{+}, firstnumber=auto, showstringspaces=false, belowcaptionskip=0em] 
Now, as an expert in linked data and knowledge engineering, please 
convert the procedure included in the json into an RDF Turtle 
formatted knowledge graph.

Using the ontology provided in the example below exclusively, please 
create from your json specific instances and data about the procedure, 
the steps of the procedure, the tools used in the steps, if any, and 
the actions mentioned in the steps. Also, create the RDF graph. 
Add labels to all instances. 

Follow best practices of Linked Data and common standard vocabularies 
as basis for the modeling unless specified differently in the 
requirements above. 
Do not extract any other properties or values than the ones I mentioned, 
but validate your output step by step, to check whether all used prefixes 
are included and the given requirements as well as the grammar of the RDF 
turtle serialization were respected.
Include only instances and data that are explicitly mentioned in the text.
Only return the turtle format, no additional text.

Include as label of the steps the actual sentence or sentences describing 
the step in the original text, without rephrasing them.

Let's use an example.

From the json I previously generated
{keyboard_actions}
I generate the RDF graph in Turtle format:
{keyboard_ttl}

The example ends here. 

Generate your RDF graph.
{actions-steps}
\end{lstlisting}

\section{Human assessment}

\subsection{Survey for human evaluation of LLM results}
\label{sec:app-eval}
This section provides more details on the questions that were asked to the participants, for evaluating the results of the procedural knowledge extraction performed by the LLM.

\begin{figure}[t]
    \centering
    \caption{Questions for the evaluation of each step, tool, and action extracted.}
    \includegraphics[width=0.8\linewidth]{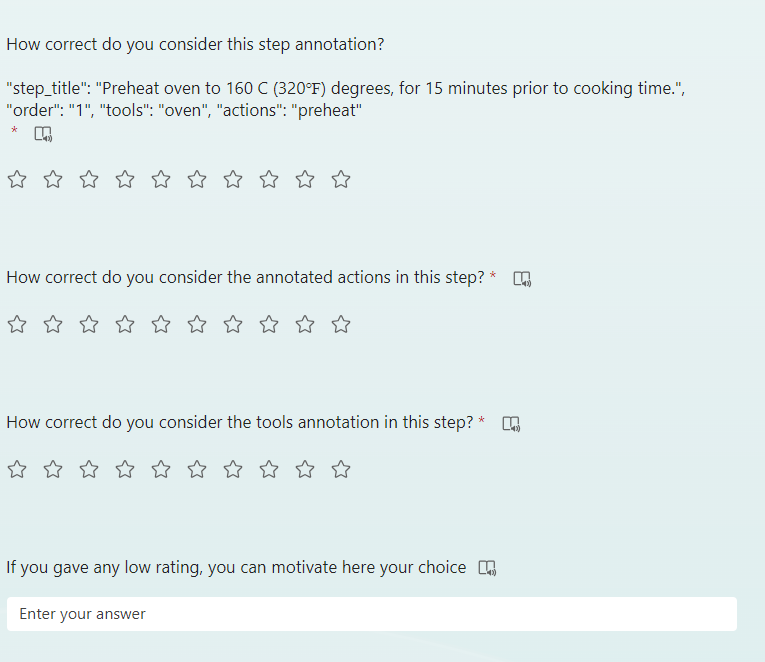}
    \label{fig:step-eval}
\vspace{\spaceunderfig}
\end{figure}

\begin{figure}[t]
    \centering
    \caption{Questions for the evaluation of the overall extraction of steps.}
    \includegraphics[width=0.8\linewidth]{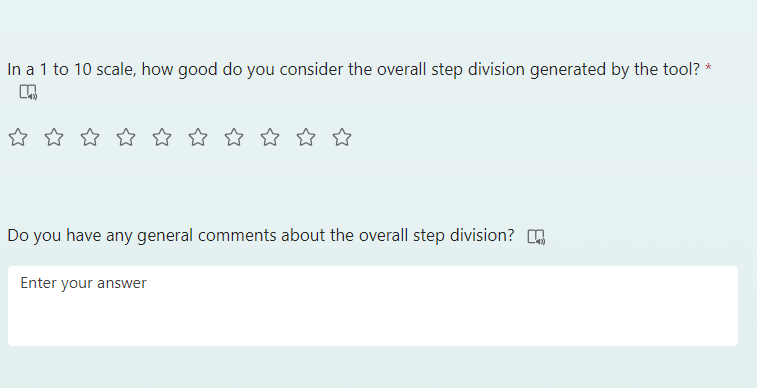}
    \label{fig:overall-step-eval}
\vspace{\spaceunderfig}
\end{figure}
